# Supplementary material for: Peak Time-Windowed Risk Estimation of Stochastic Processes
Source: arXiv:2404.06961 source file (2024-04-11)
Supplement: Supplementary file 2 [file app_risk_measures.tex]

% \section{Other Risk Measures}

% This appendix lists how 
